# Supplementary material for: A phase field model for mass transport with semi-permeable interfaces
Source: arXiv:2103.06430 source file (2021-03-11)
Supplement: Supplementary file 1 [file appendices.tex]

\appendix
\appendixpage
\addcontentsline{toc}{section}{Appendices}\markboth{APPENDICES}{}
\begin{subappendices}
\subsection{Mathematical notations used in the paper}
Mathematical notations used in this paper are follows. Suppose a 2-rank tensor is denoted as $F$, 
its $l_{2}$ norm is $|F|^{2}=\sum F_{ij}^{2}$. 
If $A$ and $B$ are two 2-rank tensors, 
then $(AB)_{ij}=\sum\limits_{k}A_{ik}B_{kj}$ and the double dot product of these two tensors is $A:B=\sum\limits_{ij}A_{ij}B_{ij}$. 
If $\bm{a}$ and $\bm{b}$ are two vectors, the outer pruduct $\bm{a}\otimes\bm{b}$ means 
$(\bm{a}\otimes\bm{b})_{ij}=\bm{a}_{i}\bm{b}_{j}$. $L^{2}$ norm of the smooth function $f$ in the domain $\Omega$, 
$(\int_{\Omega}|f|^{2}\mathrm{d}\bm{x})^{1/2}$, is denoted by $\|f\|_{\Omega}$. 
%and the $L^{2}$ norm on the boundary $w$, $(\int_{\Gamma}|f|^{2}\mathrm{d}s)^{1/2}$, is denoted by $\|f\|_{\Gamma}$. 
If $f$ and $g$ are two smooth functions in $\Omega$, 
$(f,g)$ stands for the inner product of these two functions and it is defined by $(f,g)=\int_{\Omega}fg\mathrm{d}\bm{x}$.

\subsection{Detail calculation}\label{detail calculation}
For the entropy, we have 
\begin{align}\label{eqn: entropy dissipation}
\frac{\mathrm{d}}{\mathrm{d}t}E_{ent}
&=\int_{\Omega}\mu_{c}(\frac{\partial c}{\partial t}+\bm{u}\cdot\nabla c)\mathrm{d}\bm{x}
\nonumber\\
&=-\int_{\Omega}\mu_{c}\nabla\cdot\bm{j}_{c}\mathrm{d}\bm{x}
\nonumber\\
&=-\int_{\partial\Omega}\mu_{c}\bm{j}_{c}\cdot\bm{n}\mathrm{d}\bm{x}
+\int_{\Omega}\nabla\mu_{c}\cdot\bm{j}_{c}\mathrm{d}\bm{x}
\nonumber\\
&=\int_{\Omega}\nabla\mu_{c}\cdot\bm{j}_{c}\mathrm{d}\bm{x}.
\end{align}

For the kinetic energy, we have 
\begin{align}\label{eqn: kinetic dissipation}
\frac{\mathrm{d}}{\mathrm{d}t}E_{kin}
=&\frac{\mathrm{d}}{\mathrm{d}t}(\frac{1}{2}\int_{\Omega}\rho|\bm{u}|^{2}\mathrm{d}\bm{x})
\nonumber\\
=&\frac{1}{2}\int_{\Omega}\frac{\partial\rho}{\partial t}|\bm{u}|^{2}\mathrm{d}\bm{x}
+\int_{\Omega}\rho\bm{u}\cdot\frac{\partial \bm{u}}{\partial t}\mathrm{d}\bm{x}
\nonumber\\
=&\frac{1}{2}\int_{\Omega}\frac{\partial\rho}{\partial t}|\bm{u}|^{2}\mathrm{d}\bm{x}
+\int_{\Omega}\rho\bm{u}\cdot\frac{\textbf{D}\bm{u}}{\textbf{D}t}\mathrm{d}\bm{x}
+\int_{\Omega}\nabla\cdot(\rho\bm{u})\frac{|\bm{u}|^{2}}{2}\mathrm{d}\bm{x}
\nonumber\\
=&\int_{\Omega}\bm{u}\cdot(\nabla\cdot\sigma_{\eta}+\nabla\cdot\sigma_{\phi})\mathrm{d}\bm{x}
-\int_{\Omega}p\nabla\cdot\bm{u}\mathrm{d}\bm{x}
\nonumber\\
=&-\int_{\Omega}\nabla\bm{u}:(\sigma_{\eta}+\sigma_{\phi})\mathrm{d}\bm{x}
-\int_{\Omega}p\nabla\cdot\bm{u}\mathrm{d}\bm{x}
\end{align}

For the mix energy, we have 
\begin{align*}
&\frac{\mathrm{d}}{\mathrm{d}t}\int_{\Omega}(G(\phi)+\frac{\gamma^{2}}{2}|\nabla\phi|^{2})\mathrm{d}\bm{x}\\
=&\int_{\Omega}\frac{\partial}{\partial t}(G(\phi)+\frac{\gamma^{2}}{2}|\nabla\phi|^{2})\mathrm{d}\bm{x}\\
=&\int_{\Omega}(G^{\prime}(\phi)\frac{\partial\phi}{\partial t}+\gamma^{2}\nabla\phi\cdot\frac{\partial}{\partial t}\nabla\phi)\mathrm{d}\bm{x}\\
=&\int_{\Omega}(G^{\prime}(\phi)\frac{\partial\phi}{\partial t}+\gamma^{2}\nabla\phi\cdot\nabla\frac{\partial\phi}{\partial t})\mathrm{d}\bm{x}\\
=&\int_{\Omega}G^{\prime}(\phi)\frac{\partial\phi}{\partial t}\mathrm{d}\bm{x}+\int_{\partial\Omega}\gamma^{2}\frac{\partial\phi}{\partial\bm{n}}\frac{\partial\phi}{\partial t}\mathrm{d}s-\int_{\Omega}\nabla\cdot(\gamma^{2}\nabla\phi)\frac{\partial\phi}{\partial t}\mathrm{d}\bm{x}\\
=&\int_{\Omega}(G^{\prime}(\phi)-\nabla\cdot(\gamma^{2}\nabla\phi))\frac{\partial\phi}{\partial t}\mathrm{d}\bm{x}
+\int_{\partial\Omega}\gamma^{2}\frac{\partial\phi}{\partial\bm{n}}\frac{\partial\phi}{\partial t}\mathrm{d}s\\
=&\int_{\Omega}\mu_{\phi}\frac{\partial\phi}{\partial t}\mathrm{d}\bm{x}
+\int_{\partial\Omega}\gamma^{2}\frac{\partial\phi}{\partial\bm{n}}\frac{\partial\phi}{\partial t}\mathrm{d}s\\
=&\int_{\Omega}\mu_{\phi}(\frac{\partial\phi}{\partial t}+\bm{u}\cdot\nabla\phi)\mathrm{d}\bm{x}
-\int_{\Omega}\mu_{\phi}\bm{u}\cdot\nabla\phi\mathrm{d}\bm{x}
+\int_{\partial\Omega}\gamma^{2}\frac{\partial\phi}{\partial\bm{n}}\frac{\partial\phi}{\partial t}\mathrm{d}s\\
=&-\int_{\Omega}\mu_{\phi}\nabla\cdot\bm{j}_{\phi}\mathrm{d}\bm{x}
-\int_{\Omega}\mu_{\phi}\bm{u}\cdot\nabla\phi\mathrm{d}\bm{x}
+\int_{\partial\Omega}\gamma^{2}\frac{\partial\phi}{\partial\bm{n}}\frac{\partial\phi}{\partial t}\mathrm{d}s\\
=&\int_{\Omega}\nabla\mu_{\phi}\cdot\bm{j}_{\phi}\mathrm{d}\bm{x}
-\int_{\partial\Omega}\mu_{\phi}\bm{j}_{\phi}\cdot\bm{n}\mathrm{d}s
-\int_{\Omega}(G(\phi)-\nabla\cdot(\gamma^{2}\nabla\phi))\bm{u}\cdot\nabla\phi\mathrm{d}\bm{x}
+\int_{\partial\Omega}\gamma^{2}\frac{\partial\phi}{\partial\bm{n}}\frac{\partial\phi}{\partial t}\mathrm{d}s\\
=&\int_{\Omega}\nabla\mu_{\phi}\cdot\bm{j}_{\phi}\mathrm{d}\bm{x}
-\int_{\Omega}\bm{u}\cdot \nabla G(\phi)\mathrm{d}\bm{x}
+\int_{\Omega}\gamma^{2}\Delta\phi\nabla\phi\cdot\bm{u}\mathrm{d}\bm{x}
-\int_{\partial\Omega}\mu_{\phi}\bm{j}_{\phi}\cdot\bm{n}\mathrm{d}s
+\int_{\partial\Omega}\gamma^{2}\frac{\partial\phi}{\partial\bm{n}}\frac{\partial\phi}{\partial t}\mathrm{d}s\\
=&\int_{\Omega}\nabla\mu_{\phi}\cdot\bm{j}_{\phi}\mathrm{d}\bm{x}
-\int_{\Omega}\bm{u}\cdot \nabla G(\phi)\mathrm{d}\bm{x}
+\int_{\Omega}\gamma^{2}(\nabla\cdot(\nabla\phi\otimes\nabla\phi)
-\frac{1}{2}\nabla|\nabla\phi|^{2})\cdot\bm{u}\mathrm{d}\bm{x}\\
&-\int_{\partial\Omega}\mu_{\phi}\bm{j}_{\phi}\cdot\bm{n}\mathrm{d}s
+\int_{\partial\Omega}\gamma^{2}\frac{\partial\phi}{\partial\bm{n}}\frac{\partial\phi}{\partial t}\mathrm{d}s\\
=&\int_{\Omega}\nabla\mu_{\phi}\cdot\bm{j}_{\phi}\mathrm{d}\bm{x}
-\int_{\Omega}\bm{u}\cdot \nabla (G(\phi)+\frac{\gamma^{2}}{2}|\nabla\phi|^{2})\mathrm{d}\bm{x}
+\int_{\Omega}\gamma^{2}\nabla\cdot(\nabla\phi\otimes\nabla\phi)\cdot\bm{u}\mathrm{d}\bm{x}\\
&-\int_{\partial\Omega}\mu_{\phi}\bm{j}_{\phi}\cdot\bm{n}\mathrm{d}s
+\int_{\partial\Omega}\gamma^{2}\frac{\partial\phi}{\partial\bm{n}}\frac{\partial\phi}{\partial t}\mathrm{d}s\\
=&\int_{\Omega}\nabla\mu_{\phi}\cdot\bm{j}_{\phi}\mathrm{d}\bm{x}
-\int_{\Omega}\nabla\cdot(\bm{u}(G(\phi)+\frac{\gamma^{2}}{2}|\nabla\phi|^{2}))\mathrm{d}\bm{x}
+\int_{\Omega}(G(\phi)+\frac{\gamma^{2}}{2}|\nabla\phi|^{2})\nabla\cdot\bm{u}\mathrm{d}\bm{x}\\
&+\int_{\Omega}\gamma^{2}\nabla\cdot(\nabla\phi\otimes\nabla\phi)\cdot\bm{u}\mathrm{d}\bm{x}
-\int_{\partial\Omega}\mu_{\phi}\bm{j}_{\phi}\cdot\bm{n}\mathrm{d}s
+\int_{\partial\Omega}\gamma^{2}\frac{\partial\phi}{\partial\bm{n}}\frac{\partial\phi}{\partial t}\mathrm{d}s\\
=&\int_{\Omega}\nabla\mu_{\phi}\cdot\bm{j}_{\phi}\mathrm{d}\bm{x}
-\int_{\partial\Omega}(G(\phi)+\frac{\gamma^{2}}{2}|\nabla\phi|^{2}))\bm{u}\cdot\bm{n}\mathrm{d}s
+\int_{\Omega}\gamma^{2}\nabla\cdot(\nabla\phi\otimes\nabla\phi)\cdot\bm{u}\mathrm{d}\bm{x}\\
&-\int_{\partial\Omega}\mu_{\phi}\bm{j}_{\phi}\cdot\bm{n}\mathrm{d}s
+\int_{\partial\Omega}\gamma^{2}\frac{\partial\phi}{\partial\bm{n}}\frac{\partial\phi}{\partial t}\mathrm{d}s\\
=&\int_{\Omega}\nabla\mu_{\phi}\cdot\bm{j}_{\phi}\mathrm{d}\bm{x}
-\int_{\Omega}\gamma^{2}(\nabla\phi\otimes\nabla\phi):\nabla\bm{u}\mathrm{d}\bm{x}, 
\end{align*}
where we use the incompressible condition and boundary condition 
$\bm{u}\cdot\bm{n}|_{\partial\Omega}=0,\bm{j}_{\phi}\cdot{\bm{n}}|_{\partial\Omega}=0,\frac{\partial\phi}{\partial\bm{n}}|_{\partial\Omega}=0.$

Note that
\begin{align*}
|D_{\eta}|^{2}=&\big|\frac{\nabla\bm{u}+(\nabla\bm{u})^{T}}{2}\big|^{2}\\
=&\frac{1}{4}\sum_{i,j}(\partial_{i}u_{j}+\partial_{j}u_{i})^{2}\\
=&\frac{1}{4}\sum_{i,j}\big((\partial_{i}u_{j})^{2}+(\partial_{j}u_{i})^{2}+2\partial_{i}u_{j}\partial_{j}u_{i}\big)\\
=&\frac{1}{4}\sum_{i,j}\big((\partial_{i}u_{j})^{2}+\partial_{i}u_{j}\partial_{j}u_{i}\big)
+\sum_{i,j}\big(\partial_{j}u_{i})^{2}+\partial_{i}u_{j}\partial_{j}u_{i}\big)\\
=&\frac{1}{2}\sum_{i,j}\big((\partial_{i}u_{j})^{2}+\partial_{i}u_{j}\partial_{j}u_{i}\big)\\
=&\frac{1}{2}\sum_{i,j}(\partial_{i}u_{j}+\partial_{i}u_{j}\partial_{j}u_{i})(\partial_{i}u_{j})\\
=&D_{\eta}:\nabla\bm{u}.
\end{align*}

\subsection{}
The following equation is important in derivation of this system. 
\begin{equation}\label{eqn: cross multiply}
\nabla\cdot(\nabla\phi\otimes\nabla\phi)=\Delta\phi\nabla\phi+\frac{1}{2}\nabla|\nabla\phi|^{2}. 
\end{equation}
\begin{proof}
Note that each element of $\nabla\cdot(\nabla\phi\otimes\nabla\phi)$ is 
\begin{equation*}
\partial_{j}(\partial_{i}\phi\partial_{j}\phi)
=\partial_{i}\phi\partial_{jj}^{2}\phi+\partial_{j}(\partial_{i}\phi)\partial_{j}\phi
=\partial_{i}\phi\partial_{jj}^{2}\phi+\partial_{i}(\partial_{j}\phi)\partial_{j}\phi.
\end{equation*}
\end{proof}
\end{subappendices}
